# Supplementary material for: FedDC: Federated Learning with Non-IID Data via Local Drift Decoupling and Correction
Source: arXiv:2203.11751 source file (2022-03-22)
Supplement: Supplementary file 1 [file appendix.tex]

\pagebreak
\section{appendix}

\subsection{Assumption defintions}

\textbf{(D1)} $f$ is $\beta$-continuous gradient satifies:
\begin{equation}\label{key}
||\Delta f(x)-\Delta f(y)||<=\beta||x-y||, \quad for \quad any \quad x, y.
\end{equation}	
and its implication of quadratic bound:
\begin{equation}
f(x)<=f(y)+<\Delta{f(y)},x-y>+\beta/2||x-y||^2
\end{equation}

\textbf{(D2)} $f$ is $\beta$ smooth function
\begin{equation}
||\Delta f(\theta_1)-\Delta f(\theta_2)||^2<=L||\theta_1-\theta_2||^2
\end{equation}

\textbf{(D3)} $f$ is a $\mu$-convex function 
\begin{equation}
f(y)>=f(x)+\Delta f(x)(y-x)
\end{equation}
while $\mu=1$, $f$ is strong convex,
that implies $f$ satifies Jensen’s inequality
\begin{equation}
f(E(x))<=E(f(x))
\end{equation}

\textbf{(D4)} $f$ is a $\mu$-convex function 
\begin{equation}
f(y)>=f(x)+\Delta f(x)(y-x)
\end{equation}
while $\mu=1$, $f$ is strong convex,
that implies $f$ satifies Jensen’s inequality
\begin{equation}
f(E(x))<=E(f(x))
\end{equation}

\textbf{(D5)} $g(\theta_i)$ is unbiased gradient of $f_i$'s local gradients with a bound variance
\begin{equation}
\mathbb{E}||g(\theta_i)-\delta f_i(\theta_i)||<=\sigma^2
\end{equation}

If $f_i$ is convex and $\beta$ smooth, with Jensen’s inequality and triangle inequality, we get:
\begin{equation}
\frac{1}{2\beta m}\sum_{i=0}^m||\Delta f_i(x)-\Delta f_i(y)||^2 <= ||\sum_{i=0}^mf_i(x)-\sum_{i=0}^mf_i(y)||
\end{equation}
\begin{equation}
<\Delta f(x),y-z><= f(y)-f(z)+\frac{\beta}{2} ||z-x||^2 \quad, \quad \forall x,y,z
\end{equation}

\subsection{Proof of client drift in FedAVG \ref{}}
With the assumption of the loss function $l(\theta,(x,y))$ is $\lambda$-Lipschitz continuous gradient, we have 
\begin{equation}\label{key}
||\frac{\partial{l(\theta,(x,y))}}{\partial\theta_1}-\frac{\partial{l(\theta,(x,y))}}{\partial\theta_2}||<=\lambda||\theta_1-\theta_2||
\end{equation}
Compute the divation between the unbias parameter form centrilized training and the parameter from FedAVG in round $t$ intertion $K$:

\begin{equation}{\label{appendix1}}
\begin{split}
&||\theta^{f}(t,K)-\theta^{c}(t,K)||\\
&= ||\sum_{i=1}^m\frac{1}{m}\theta_i^f(t,K)-\theta^c(t,K)||\\
&=||(\sum_{i=1}^m\frac{1}{m}\theta_i^f(t,K-1)-\eta\sum_{j=1}^CP_i(y=j)E_{x|y=j}\frac{\partial{l(\theta^f(t,K-1),(x,y=j))}}{\partial\theta^f(t,K-1)})\\
& \quad -(\theta^c(t,K-1)-\eta\sum_{j=1}^CP(y=j)E_{x|y=j}\frac{\partial{l(\theta^c(t,K-1),(x,y=j))}}{\partial\theta^c(t,K-1)} )||\\
&<= ||(\sum_{i=1}^m\frac{1}{m}\theta_i^f(t,K-1)-\theta^c(t,K-1)||\\
& \quad +\eta||\sum_{j=1}^CP(y=j)E_{x|y=j}\frac{\partial{l(\theta^c(t,K-1),(x,y=j))}}{\partial\theta^c(t,K-1)}-\sum_{j=1}^CP_i(y=j)E_{x|y=j}\frac{\partial{l(\theta^f(t,K-1),(x,y=j))}}{\partial\theta^f(t,K-1)}||\\
&<=\sum_{i=1}^m\frac{1}{m}(1+\eta\sum_{j=1}^CP_i(y=j)\lambda)||\theta_i^f(t,K-1)-\theta^c(t,K-1)||
\end{split}
\end{equation}

Calculate the divation between unbias gradients form centrilized training and the client $i$'s gradient in round $t$ intertion $K$, we get:
\begin{equation}{\label{appendix2}}
\begin{split}
&||\sum_{j=1}^CP_i(y=j)E_{x|y=j}\frac{\partial{l(\theta_i^f(t,K),(x,y=j))}}{\partial\theta_i^f(t,K)} -\sum_{j=1}^CP(y=j)E_{x|y=j}\frac{\partial{l(\theta^c(t,K),(x,y=j))}}{\partial\theta^c(t,K)}||\\
&= ||\sum_{j=1}^CP_i(y=j)E_{x|y=j}\frac{\partial{l(\theta_i^f(t,K),(x,y=j))}}{\partial\theta_i^f(t,K)} -\sum_{j=1}^CP(y=j)E_{x|y=j}\frac{\partial{l(\theta^c(t,K),(x,y=j))}}{\partial\theta^c(t,K)}\\
&\quad -(\sum_{j=1}^CP_i(y=j)E_{x|y=j}\frac{\partial{l(\theta^c(t,K),(x,y=j))}}{\partial\theta^c(t,K)}+\sum_{j=1}^CP_i(y=j)E_{x|y=j}\frac{\partial{l(\theta^c(t,K),(x,y=j))}}{\partial\theta^c(t,K)})||\\
&<= ||\sum_{j=1}^CP_i(y=j)E_{x|y=j}\frac{\partial{l(\theta_i^f(t,K),(x,y=j))}}{\partial\theta_i^f(t,K)}-\frac{\partial{l(\theta^c(t,K),(x,y=j))}}{\partial\theta^c(t)}||\\
& \quad +||\sum_{j=1}^C(P_i(y=j)-P(y=j))E_{x|y=j}\frac{\partial{l(\theta^c(t,K),(x,y=j))}}{\partial\theta^c(t,K)}||
\end{split}
\end{equation}

Taking $\Psi(\theta)=max_{j=1}^C||\frac{\partial{l(\theta,(x,y=j))}}{\partial\theta}||$ and the conclusion of Equation \ref{appendix2}, we can calculate the divation between unbias parameter form centrilized training and the client $i$'s parameter in round $t$ interation $K-1$:
\begin{equation}{\label{appendix3}}
\begin{split}
&||\theta_{i}^f(t,K-1)-\theta^{c}(t,K-1)||\\
&=||(\theta_i^f(t,K-2)-\eta\sum_{j=1}^CP_i(y=j)E_{x|y=j}\frac{\partial{l(\theta_i^f(t,K-2),(x,y=j))}}{\partial\theta_i^f(t,K-2)})\\
& \quad -(\theta^c(t,K-2)+\eta\sum_{j=1}^CP(y=j)E_{x|y=j}\frac{\partial{l(\theta^c(t,K-2),(x,y=j))}}{\partial\theta^c(t,K-2)} )||\\
&<= ||(\theta_i^f(t,K-2)-\theta^c(t,K-2)||\\
& \quad +\eta||\sum_{j=1}^CP_i(y=j)E_{x|y=j}\frac{\partial{l(\theta_i^f(t,K-2),(x,y=j))}}{\partial\theta_i^f(t,K-2)}-\sum_{j=1}^CP(y=j)E_{x|y=j}\frac{\partial{l(\theta^c(t,K-2),(x,y=j))}}{\partial\theta^c(t,K-2)}||\\
&<=(1+\eta\sum_{j=1}^CP_i(y=j))||\theta_i^f(t,K-2)-\theta^c(t,K-2)||+\eta\Psi(\theta^c(t,K-2))\sum_{j=1}^C||P_i(y=j)-P(y=j)||
\end{split}
\end{equation}

Taking $\alpha_i=1+\eta\sum_{j=1}^CP_i(y=j)\lambda{x|y=j}>1$ and Equation \ref{appendix2} into Equation \ref{appendix3}:
\begin{equation}{\label{appendix3}}
\begin{split}
&||\theta_{i}^f(t,K-1)-\theta^{c}(t,K-1)||\\
&<=\alpha_i||\theta_i^f(t,K-2)-\theta^c(t,K-2)||+\eta\Psi(\theta^c(t,K-2))\sum_{j=1}^C||P_i(y=j)-P(y=j)||\\
&<= (\alpha_i)^2||\theta_i^f(t,K-3)-\theta^c(t,K-3)||+\eta\sum_{j=1}^C||P_i(y=j)-P(y=j)||(\Psi(\theta^c(t,K-2))+\alpha_i\Psi(\theta^c(t,K-3)))\\
&<=(\alpha_i)^{K-1}||\theta_i^f(t-1,K)-\theta^c(t-1,K)||+\eta\sum_{j=1}^C||P_i(y=j)-P(y=j)||(\sum_{k=0}^{K-2}(\alpha_i)^{k}\Psi(\theta^c(t-1,K-2-k)))
\end{split}
\end{equation}

so that with Equation \ref{appendix1} and Equation \ref{appendix3} proved,

\begin{equation}{\label{lamma}}
\begin{split}
||\theta^f(t,K)-\theta^c(t,K)|&<=\sum_{i=1}^m\frac{1}{m}(1+\eta\sum_{j=1}^CP_i(y=j)\lambda)||\theta_i^f(t,K-1)-\theta^c(t,K-1)||\\
&<=\sum_{i=1}^m\frac{1}{m}((\alpha_i)^K||\theta^f(t-1,K)-\theta^c(t-1,K)||\\
&+\eta\sum_{i=1}^m\frac{1}{m}\sum_{j=1}^C||P_i(y=j)-P(y=j)||\sum_{k=0}^{K-1}(\alpha_i)^k\Psi({\theta^c(t,K-1-i)}))
\end{split}
\end{equation}

\subsection{FedAutoOp convenge analysis}

\textbf{parameter upodate}
\begin{equation}{\label{lamma}}
\Theta=\Theta+\Delta \Theta =\Theta+h_g \quad where \quad \Theta=\theta+h \quad and \quad h_g^t=\Delta\Theta-h_g^{t-1}=\Delta\theta+ \Delta h = h_g^{t-1}+\Delta\theta+ \Delta h 
\end{equation}

\textbf{Assumption}

\textbf{Definiitions}
\begin{equation}{\label{lamma}}
C_t=\frac{1}{m}\sum_{i=1}\sum_{k=1}({\frac{\partial L_i}{\partial \theta_i^k} +\frac{\partial L_i}{\partial h_i^k}})
\end{equation}

\begin{equation}{\label{lamma}}
D_i^t=\frac{1}{M}\sum_{i=1}\sum_{k=1}||h_g^t-\Delta L_i(\Theta^*)||^2
<=(1-S/M)D_{t-1}+ 2/(M^2k)\sum{k=1}E||\Delta L_i(\Theta_{i}^{k})||^2
\end{equation}

\begin{equation}{\label{lamma}}
D^t=E(D_i^t)
<=(1-S/M)D_{t-1}+ 2/(M^2k)\sum{k=1,m=1}E||\Delta L_i(\Theta_{i}^{k})||^2
\end{equation}

\section{Client drift in one round}
Assuming $\theta_c^{t-1}=\theta_i^{t-1}$, and $||\delta L(\theta)-\delta L_i(\theta)||\leq \sigma$, $||\delta L_i(\theta_1)-\delta L_i(\theta_2)||<=\beta||\theta_1-theta_2||$
\begin{equation}{\label{lamma}}
\begin{split}
&||\Delta \theta_c^t-\Delta \theta_i^t||=\\
&=||\sum_{k=1}^K{\delta L(\theta_c^{t,k}) }-\sum_{k=1}^K{\delta L_i(\theta_c^{t,k}) }||\\
&=||\sum_{k=1}^K{\delta L(\theta_c^{t,k}) }-\sum_{k=1}^K{\delta L_i(\theta_c^{t,k}) }+\sum_{k=1}^K{\delta L_i(\theta_c^{t,k}) }-\sum_{k=1}^K{\delta L_i(\theta_i^{t,k}) }||\\
&<=K\sigma+\sigma+(1+\beta)\sigma+(1+\beta)^2\sigma+...+(1+\beta)^{K-1}\sigma\\
&<=K\sigma+\frac{(1+\beta)^k-1}{\beta}\sigma
\end{split}
\end{equation}

\section{Update of FedAutoOp}
Local update\\
\begin{equation}{\label{lamma}}
\theta_{i,k+1}=\theta_{i,k}-\eta g(\theta_{i,k}), \quad where \quad 
g(\theta_{i,k})= \delta \theta_{i,k}+\alpha(h_i-\Theta)+ c-c_i
\end{equation}
Global update:\\
where the control variable:
\begin{equation}{\label{lamma}}
h_i^r=h_i^{r-1}+\Delta{\theta_i^r}, \quad c_i^r=c^{r-1}-c_i^{r-1}+\frac{1}{K\eta}(\theta_i^{r-1}-\theta_i^{r,K}), \quad c^r=\mathbb{E}c_i^r
\end{equation}

the global parameter:
\begin{equation}{\label{lamma}}
\Theta^r=\Theta^{r-1}+h+\Delta h+\Delta \theta=\mathbb{E}_{{i\in S_r}}(\theta_i^r+h_i^r) 
\end{equation}

\subsection{Defination}
\begin{equation}{\label{lamma}}
\Theta^r=\Theta^{r-1}+\Delta h+h+\Delta \theta=\mathbb{E}_{{i\in S_r}}(\theta_i^r+h_i^r) 
\end{equation}

\section{Lamma: Bound the variance of the server update}
\begin{equation}{\label{lamma}}
\mathbb{E}\left\|\Theta^r-\Theta^{r-1}\right\|\leq ??? 
\end{equation}
\begin{equation}{\label{lamma}}
\Theta^r=\Theta^{r-1}+2\Delta \theta_r +2\alpha
\end{equation}

The global update in round $r$ as:
\begin{equation}{\label{lamma}}
\begin{split}
&\mathbb{E} \left\|\Delta \Theta\right\|^2
=\mathbb{E}\left\|h-2\frac{\eta}{KS}g(\theta_{i,k})\right\|^2
=\mathbb{E}\left\|\frac{1}{S}\sum_{S}h_i-2\frac{\eta}{KS}\sum_{S}(\delta \theta_{i,k}+\alpha(h_i-\Theta)+ c-c_i)\right\|^2\\
&\leq 2\mathbb{E} \left\|\frac{1}{S}\sum_{S}h_i\right\|^2+8\mathbb{E} \left\| \frac{\eta}{KS}\sum_{S}(\delta \theta_{i,k}+\alpha(h_i-\Theta)+ c-c_i) \right\|^2\\
\end{split}
\end{equation}

\pagebreak

\section{Imitate the Proof of FedProx}
\textbf{Assumption 1.} $f$ is $\beta$-smoothness means 
\begin{equation}{\label{lammap1}}
||\nabla f(\theta_1)-\nabla f(\theta_2)||\leq \beta ||\theta_1-\theta_2||, \forall \theta_1,\theta_2
\end{equation}  

In FLN, the parameter of global model consists of average of local model parameter and average of local parameter deviation.
\begin{equation}{\label{lammap1}}
\Theta=\mathbb{E}_i(\theta_i+h_i)=\mathbb{E}_i\theta_i+\mathbb{E}_ih_i
\end{equation}
For the corrected local paraeter
\begin{equation}{\label{lammap1}}
\hat\theta_i^t=\Theta^t-h_i^t, \quad
\mathbb{E}\hat\theta_i^t=\Theta^t-\mathbb{E}h_i^t=\mathbb{E}_i\theta_i^t
\end{equation}
Local objective function
\begin{equation}{\label{lammap1}}
F_i(\theta_i)=L_i(\theta_i)+\frac{\alpha}{2}||\theta_i-\hat\theta_i^t||^2
\end{equation}
so that $\theta_i^{t+1}$ satifies
\begin{equation}{\label{lammap1}}
\nabla F_i(\theta_i^{t+1})=\nabla L_i(\theta_i^{t+1})+ \alpha(\theta_i^{t+1}-\hat\theta_i^t)
\end{equation}
\begin{equation}{\label{lammap1}}
\mathbb{E}_i\nabla F_i(\theta_i^{t+1})=\mathbb{E}_i\nabla L_i(\theta_i^{t+1})+ \alpha \mathbb{E}_i(\theta_i^{t+1}-\hat\theta_i^t), \qquad
\mathbb{E}_i\nabla F_i(\theta_i^{t+1})=\mathbb{E}_i\nabla L_i(\theta_i^{t+1})+ \alpha \mathbb{E} (\theta^{t+1}-\theta^t)
\end{equation}
that is 
\begin{equation}{\label{lammap1}}
\theta^{t+1}-\theta^t=\frac{1}{\alpha}(\mathbb{E}_i\nabla F_i(\theta_i^{t+1})-\mathbb{E}_i\nabla L_i(\theta_i^{t+1}))
\end{equation}
In addition
\begin{equation}{\label{lammap1}}
h_i^{t+1}=h_i^t+\theta_i^{t+1}-\theta_i^t, \quad and \quad \theta^{t+1}-\theta^t=\frac{1}{\alpha}(\mathbb{E}_i\nabla F_i(\theta_i^{t+1})-\mathbb{E}_i\nabla L_i(\theta_i^{t+1}))
\end{equation}
so that 
\begin{equation}{\label{lammap1}}
\Theta^{t+1}-\Theta^{t+1}=\mathbb{E} (h_i^{t+1}-h_i^t+\theta_i^{t+1}-\theta_i^t)=2(\theta^{t+1}-\theta^t)
\end{equation}

\textbf{Assumption 2.}
If $\theta_i^*$ is a $\gamma$-inexact solution of $F_i(\theta_i,\hat{\theta_i})$ and
\begin{equation}{\label{lammap1}}
F_i(\theta_i,\hat{\theta_i})=L_i(\theta_i)+\frac{\alpha}{2}||\theta_i-\hat\theta_i||^2
\end{equation}
then
\begin{equation}{\label{lammap2}}
||\nabla F_i(\theta_i^*,\hat{\theta_i})||
 \leq \gamma||\nabla F_i(\hat{\theta_i},\hat{\theta_i})||
\end{equation}
\begin{equation}{\label{lammap3}}
\nabla F_i(\theta_i,\hat{\theta_i}) = \nabla L_i(\theta_i) + \alpha (\theta_i-\hat\theta_i)
\end{equation}

\textbf{Proof from here}

In the proof, we follow the techniques of \cite{li2020federated}.
Define $e_i^{t}$ as
\begin{equation}{\label{lammap4}}
\nabla L_i(\theta_i^t) + \alpha (\theta_i^t-\hat\theta_i^{t-1}) -e_i^t=0
\end{equation}
We have $\nabla F_i(\hat\theta_i^{t-1},\hat\theta_i^{t-1}) = \nabla L_i(\hat\theta_i^{t-1}) $, so
\begin{equation}{\label{lammap5}}
e_i^t	\leq	\gamma||\nabla L_i(\hat\theta_i^{t-1})||
\end{equation}

Let $\bar\theta^t=\mathbb{E}_i{\theta_i^t}$ and $\bar\theta^{t-1}=\mathbb{E}_i{\hat\theta_i^t}$, we have
\begin{equation}{\label{lammap6}}
\theta_i^t-\hat\theta_i^{t-1}=\frac{1}{\alpha}(-\nabla L_i(\theta_i^{t})+e_i^{t})
\end{equation}
\begin{equation}{\label{lammap7}}
\bar\theta^t-\bar\theta^{t-1}=\mathbb{E}_i\theta_i^t-\mathbb{E}_i\hat\theta_i^{t-1}=\frac{1}{\alpha}\mathbb{E}_i(-\nabla L_i(\theta_i^{t})+e_i^{t})
\end{equation}

Let $\bar\alpha=\alpha-L_d>0$ and $\ddot\theta_i^{t}=\arg\min_\theta F_i(\theta,\hat\theta_i^{t-1})$. Due to $\bar\alpha$ convex of $F_i$, we get

\begin{equation}{\label{lammap8}}
||\ddot\theta_i^t-\theta_i^t|| \leq \frac{\gamma}{\bar\alpha}||\nabla L_i(\hat\theta_i^{t-1})||
\end{equation}
Due to $\bar\alpha$ convex of $F_i$ again, we get
\begin{equation}{\label{lammap9}}
||\ddot\theta_i^t-\hat\theta_i^{t-1}|| \leq \frac{1}{\bar\alpha}||\nabla L_i(\hat\theta_i^{t-1})||
\end{equation}
Using tringle inquality:
\begin{equation}{\label{lammap10}}
||\theta_i^t-\hat\theta_i^{t-1}|| \leq \frac{1+\gamma}{\bar\alpha}||\nabla L_i(\hat\theta_i^{t-1})||
\end{equation}
so that, with the bounded dissimilarity assumption, %\textcolor{red}{different with FedProx} 
let $\mathbb{E}\hat\theta_i^{t-1}=\hat\theta^{t-1}=\bar\theta_i^{t-1}$,
\begin{equation}{\label{lammap11}}
\begin{split}
&||\bar\theta^t-\hat\theta^{t-1}|| =||\mathbb{E}_i\theta_i^t-\mathbb{E}_i\hat\theta_i^{t-1}||
\leq \mathbb{E}_i||\theta_i^t-\hat\theta_i^{t-1}|| 
\leq \frac{1+\gamma}{\bar\alpha}\mathbb{E}_i||\nabla L_i(\hat\theta_i^{t-1})|| \\
&\leq_1 \frac{1+\gamma}{\bar\alpha}\sqrt{\mathbb{E}_i||\nabla L_i(\hat\theta_i^{t-1})||^2}
\leq_2 B\frac{1+\gamma}{\bar\alpha} ||\nabla L(\hat\theta^{t-1})||
\end{split}
\end{equation}
where the last is due to the bounded dissimilarity assumption.

Define $M_{t}$ as $\bar\theta^t-\hat\theta^{t-1}=\frac{-1}{\alpha}(\nabla L(\hat\theta^{t-1})+M_t))$, taking Equation \ref{lammap40}, so $M_t=\mathbb{E}_i[(\nabla L_i(\theta^{t})-\nabla L_i (\hat\theta^{t-1})-e_i^t]$. $M_t$ is bounded with
\begin{equation}{\label{lammap12}}
||M_t||
\leq \mathbb{E}_i[(\nabla L ||\theta^{t}-\hat\theta^{t-1}||+||e_i^t||]
\leq (\frac{L(1+\gamma)}{\bar \alpha}+\gamma)\mathbb{E}_i||\nabla L_i(\hat\theta^{t-1}) ||
\leq (\frac{L(1+\gamma)}{\bar \alpha}+\gamma)B||\nabla L(\hat\theta^{t-1}) ||
\end{equation}
The last is due to bounded dissimilarity assumption. 

Because $h_i^t=h_i^{t-1}+\Delta \theta_i^t$, we get $\mathbb{E}(\theta_i^t-\theta_i^{t-1})=\mathbb{E}(h_i^t-h_i^{t-1})=\mathbb{E}(\bar\theta^t-\ddot\theta^{t-1})$.

$\Theta^t-\Theta^{t-1}=\mathbb{E}(\theta_i^t+h_i^t)-\mathbb{E}(\theta_i^{t-1}+h_i^{t-1})=2\mathbb{E}(\theta_i^t-\theta_i^{t-1})$

With L-Lipschitz smoothness of $L$ and Taylor expansion

%\begin{equation}{\label{lamma}}
%L_i(\theta_i^{t})
%\leq L_i(\theta_i^{t-1})+<\nabla L_i(\theta_i^{t-1}), \theta_i^t-\theta_i^{t-1}>+\frac{L}{2}|| \theta_i^t-\theta_i^{t-1}||
%\leq 
%\end{equation}

\begin{equation}{\label{lammap13}}
\begin{split}
&L(\Theta^{t})
\leq L(\Theta^{t-1})+<\nabla L(\Theta^{t-1}), \Theta^t-\Theta^{t-1}>+\frac{L}{2}|| \Theta^t-\Theta^{t-1}||^2 \\
&\leq_1 L(\Theta^{t-1})+<\nabla L(\theta^{t-1}), 2\mathbb{E}(\theta_i^t-\theta_i^{t-1})>+\frac{L}{2}||2\mathbb{E}(\theta_i^t-\theta_i^{t-1})||^2\\
&\leq L(\Theta^{t-1})-\frac{2}{\alpha}||\nabla L(\theta^{t-1})||^2-\frac{2}{\alpha}<\nabla L(\theta^{t-1}),M_t >+2L\frac{B^2(1+\gamma)^2}{\hat\alpha^2}||\nabla L(\theta^{t-1})||^2\\
&\leq L(\Theta^{t-1})-(\frac{2-2\gamma B}{\alpha}-\frac{2LB(1+\gamma)}{\alpha\bar\alpha}-2L\frac{B^2(1+\gamma)^2}{\hat\alpha^2})||\nabla L(\theta^{t-1})||^2
\end{split}
\end{equation}
where $\leq_1$ is due to $\Theta=\theta^{t+1}+h^{t+1}$.

\textbf{Proof for part participantion}

With Lipschitz continuity assumption
\begin{equation}{\label{lammap14}}
L(\theta^t)\leq L(\bar\theta^t)+L_l||\theta^t-\bar\theta^t||
\end{equation}
where
\begin{equation}{\label{lammap15}}
L_l \leq ||\nabla L(\theta^{t-1})||+L \max(||\bar\theta^t-\theta^{t-1}||,||\theta^t-\theta^{t-1}||)
\leq ||\nabla L(\theta^{t-1})||+L (||\bar\theta^t-\theta^{t-1}||+||\theta^t-\theta^{t-1}||)
\end{equation}

so that we need to bound 

\begin{equation}{\label{lammap16}}
\mathbb{E}_{S_t}L(\theta^t)\leq L(\bar\theta^t)+\mathbb{E}_{S_t}L_l||\theta^t-\bar\theta^t||
\end{equation}
\begin{equation}{\label{lammap16-1}}
\mathbb{E}_{S_t}L(\Theta^t)\leq L(\bar\Theta^t)+\mathbb{E}_{S_t}L_l||\Theta^t-\bar\Theta^t||
\leq L(\bar\Theta^t)+2\mathbb{E}_{S_t}L_l||\theta^t-\bar\theta^t||
\end{equation}

\begin{equation}{\label{lammap17}}
\begin{split}
&\mathbb{E}_{S_t}L_l||\theta^t)-\bar\theta^t|| 
\leq \mathbb{E}_{S_t}[(||\nabla L(\theta^{t-1})||+L (||\bar\theta^t-\theta^{t-1}||+||\theta^t-\theta^{t-1}||)||\theta^t-\bar\theta^t|| ]\\
&\leq (||\nabla L(\theta^{t-1})||+L (||\bar\theta^t-\theta^{t-1}||)\mathbb{E}_{S_t}||\theta^t-\bar\theta^t||
+\mathbb{E}_{S_t}||\theta^t-\bar\theta^t||^2
\end{split}
\end{equation}

Taking $\mathbb{E}(\theta_i^t-\theta_i^{t-1})
\leq B\frac{1+\gamma}{\bar\alpha} ||\nabla L(\hat\theta^{t-1})||$,
\begin{equation}{\label{lamma18}}
\mathbb{E}_{S_t}||\theta^t-\bar\theta^{t}||\leq \sqrt{\mathbb{E}_{S_t}||\theta^t-\bar\theta^{t}||^2}
\end{equation}

moreover

\begin{equation}{\label{lammap19}}
\begin{split}
&\mathbb{E}_{S_t}||\theta^t-\bar\theta^{t}||^2 \leq\frac{1}{m}\mathbb{E}_{i}(||\theta_i^t-\bar\theta^{t}||^2)\\
&\leq \frac{2}{m}\mathbb{E}_{i}||\theta_i^t-\theta^{t-1}||^2, (\bar\theta^t=\mathbb{E}\theta_i^t)\\
&\leq \frac{2}{m}\frac{(1+\gamma)^2}{\bar\alpha^2}\mathbb{E}_i||\nabla L_i(\theta^{t-1})||^2, from (\ref{lammap10})\\
&\leq \frac{2B^2(1+\gamma)^2}{m\bar\alpha^2}||\nabla L(\theta^{t-1})||^2, 
\end{split}
\end{equation}
last one is due to bounded dissimilarity assumption. Replace the bound in \ref{lammap19}

\begin{equation}{\label{lammap20}}
\mathbb{E}_{S_t}L_l||\theta^t-\bar\theta^t|| \leq (\frac{B\sqrt{2}(1+\gamma)}{\bar\alpha \sqrt{m}}+\frac{LB^2(1+\gamma)^2}{\bar\alpha^2 m}(2*\sqrt{2}+2))||\nabla L(\theta^{t-1})||^2
\end{equation}

Combine \ref{lammap13},\ref{lammap16},\ref{lammap20}, we get 
\begin{equation}{\label{lammap21}}
\begin{split}
&\mathbb{E}_{S_t} L(\Theta^t)\leq L(\Theta^{t-1})-2(\frac{1}{\alpha}-\frac{\gamma}{\alpha}-\frac{B(1+\gamma)\sqrt{2}}{\bar\alpha \sqrt{m}}-\\
&\frac{LB(1+\gamma)}{\alpha\bar\alpha}-\frac{L(1+\gamma)^2B^2}{2\bar\alpha^2}-\frac{LB^2(1+\gamma)^2(2*\sqrt{2}+2)}{\bar\alpha^2 m})||\nabla L(\theta^{t-1})||^2
\end{split}
\end{equation}

\textbf{Bounded dissimilarity}
There existing $B_c$ for $c>0$ satifies $||\nabla L(\theta)||^2>c, B(\theta)\leq B_c$, where $B(\theta)=\sqrt{\frac{\mathbb{E}_i ||\nabla L_i(\theta)||^2}{||\nabla L(\theta)||^2}}$. 

\textbf{Bounded Variance}
If
\begin{equation}{\label{lammap22}}
\mathbb{E}||\nabla L_i(\theta)-\nabla L(\theta)||^2\leq \sigma^2,
\end{equation}
Then $B_c\leq \sqrt{1+\frac{\sigma^2}{c}},\quad \forall c>0$.

proof
\begin{equation}{\label{lammap23}}
\begin{split}
&\mathbb{E}||\nabla L_i(\theta)||-||\nabla L(\theta)||^2 \leq \mathbb{E}||\nabla L_i(\theta)-\nabla L(\theta)||^2\leq \sigma^2\\
&\mathbb{E}||\nabla L_i(\theta)||^2\leq \sigma^2+||\nabla L(\theta)||^2\\
&B_c=(\frac{(\mathbb{E}_i ||\nabla L_i(\theta)||^2)}{||\nabla L(\theta)||^2})^\frac{1}{2}\leq(1+\frac{\sigma^2}{c})
\end{split}
\end{equation}

\textbf{Non-convex convergence}

\textbf{Assumption:B-local dissimilarity}
If $L_i$ is non-convex, L-Lipschitz smooth, existing $L_d$ makes $\nabla^2 L_i\geq -L_d-I$ and $\bar\alpha=\alpha-L_d>0$. $B(\theta)\leq B$ if $\alpha,m,\gamma$ satisfy:
\begin{equation}{\label{lammap24}}
p=(\frac{\gamma}{\alpha}-\frac{B(1+\gamma)\sqrt{2}}{\bar\alpha \sqrt{m}}-\frac{LB(1+\gamma)}{\alpha\bar\alpha}-\frac{L(1+\gamma)^2B^2}{2\bar\alpha^2}-\frac{LB^2(1+\gamma)^2(2*\sqrt{2}+2)}{\bar\alpha^2 m})>0
\end{equation}
and 
\begin{equation}{\label{lammap25}}
\begin{split}
&\mathbb{E}_{S_t} L(\Theta^t)\leq L(\Theta^{t-1})-2p||\nabla L(\theta^{t-1})||^2
\end{split}
\end{equation}

\textbf{Convex convergence}
In convex case, $L-=0,\bar\alpha=\alpha$, if $\gamma=0$, $B\leq \sqrt{m}$ and $1<<B \leq 0.5\sqrt{m}$, we get 

%\begin{equation}{\label{lammap26}}
%\begin{split}
%&\mathbb{E}_{S_t} L(\Theta^t)\leq L(\Theta^{t-1})-(\frac{1}{\alpha}-\frac{3LB^2}{\alpha^2})||\nabla L(\theta^{t-1})||^2
%\end{split}
%\end{equation}

\begin{equation}{\label{lammap26}}
\begin{split}
&\mathbb{E}_{S_t} L(\Theta^t)\leq L(\Theta^{t-1})-2(
\frac{1-\frac{\sqrt{2}B}{\sqrt{m}}}{\alpha}-\frac{B+(\frac{(2\sqrt{2}+2)}{m}+\frac{1}{2})LB^2}{\alpha^2})||\nabla L(\theta^{t-1})||^2
\end{split}
\end{equation}

\begin{equation}{\label{lammap27}}
\begin{split}
&\mathbb{E}_{S_t} L(\Theta^t)\leq L(\Theta^{t-1})-(\frac{1}{\alpha}-\frac{3LB^2}{\alpha^2})||\nabla L(\theta^{t-1})||^2
\end{split}
\end{equation}

If $0<\alpha \leq 6LB^2$

\begin{equation}{\label{lammap28}}
\begin{split}
&\mathbb{E}_{S_t} L(\Theta^t)\leq L(\Theta^{t-1})-\frac{1}{12LB^2}||\nabla L(\theta^{t-1})||^2
\end{split}
\end{equation}
%\begin{equation}{\label{lammap29}}
%\begin{split}
%&\mathbb{E}_{S_t} L(\Theta^t)- L(\Theta^{0}) \leq -\sum_{t}\frac{1}{12LB^2}||\nabla L(\theta^{t-1})||^2\\
%& \mathbb{E}_{S_t}T||\nabla L(\theta^{t})||^2 
%\leq 12LB^2 [L(\Theta^{0}) -\mathbb{E}_{S_t} L(\Theta^T)]
%\end{split}
%\end{equation}

That spend $O(\frac{LB^2(L(\theta^*)-L(\Theta^0))}{c})$ to achieve convengence where the gradient less than $c$.

\section{FLN Convergence Proof}
\textbf{Convex assumption}
\textbf{$\beta$ smoothness assumption}
\begin{equation}{\label{lammafa1}}
||\theta_1-\theta_2||_2\leq D,\quad \forall \theta_1,\theta_2
\end{equation}
\textbf{Variable bounded assumption}
\begin{equation}{\label{lammafa2}}
||g||_2\leq G,\quad \forall G
\end{equation}
\textbf{Gradient bounded assumption}

\textbf{Analysis on FLN.}
The algorithm flow of FLN gives
\begin{equation}{\label{lammaf1}}
\Theta^t=\mathbb{E}\theta_i^t+\mathbb{E}h_i, \quad \hat\theta_i^t=\Theta^t-h_i^t, \quad \Delta \theta_i^{t+1}=\theta_i^{t+1,k}-\theta_i^{t+1,0}=\theta_i^{t+1}-\Theta^t
\end{equation}
In order to reduce symbol abuse, we use $\theta_i^t$ to replace $\theta_i^{t,k}$ below without causing confusion.

We define $F_i(\theta_i)= \mathbb{E}_{(x,y)\in D_i}l(\theta_i,(x,y)) +\frac{1}{K\eta} \langle\theta_i,\Delta\theta_i^{t-1}-\Delta\theta^{t-1}\rangle,$, define $\hat\theta_i^{t}=\Theta^t-h_i^t$ and 
\begin{equation}{\label{lammaf2}}
\dot\theta_i^{t+1}=\arg\min_{\theta_i} L_i(\theta_i) =F_i(\theta_i)+\frac{\alpha}{2} ||\theta_i-\hat{\theta}_i^{t}||^2
\end{equation}
If $i\in C_t$, we get $\theta_i^t=\dot\theta_i^t$ where $\dot\theta_i^t$ is independent with $C_t$. The first order condition of \ref{lammaf2} satifies
\begin{equation}{\label{lammaf3}}
\nabla_{\theta_i} F_i(\dot\theta_i^{t+1})=-\alpha(\dot\theta_i^{t+1}-\hat{\theta}_i^{t}), \qquad \forall i\in C_{t+1}.
\end{equation}
From the Equation \ref{lammaf1} and \ref{lammaf3}, we get 
\begin{equation}{\label{lammaf4}}
\hat{\theta}_i^{t}=\Theta^t-h_i^t=\theta_i^{t+1}+\frac{1}{\alpha} \nabla_{\theta_i} F_i(\dot\theta_i^{t+1})
\end{equation} 
With Equation \ref{lammaf1} and \ref{lammaf4}, we get 
\begin{equation}{\label{lammaf5}}
\begin{split}
\Delta \theta_i^{t+1}&=\theta_i^{t+1}-\Theta^t=\theta_i^{t+1}-(\hat{\theta}_i^{t}+h_i^t)\\
&=\theta_i^{t+1}-(\theta_i^{t+1}+\frac{1}{\alpha} \nabla_{\theta_i} F_i(\theta_i^{t+1})+h_i^t)\\
&=-(\frac{1}{\alpha} \nabla_{\theta_i} F_i(\theta_i^{t+1})+h_i^t)
\end{split}
\end{equation}
From Equation \ref{lammaf1} and \ref{lammaf5}, we get 
\begin{equation}{\label{lammaf6}}
h_i^{t+1}=h_i^t+\Delta \theta_i^{t+1}=-\frac{1}{\alpha} \nabla_{\theta_i} F_i(\theta_i^{t+1})
\end{equation}
so that 
\begin{equation}{\label{lammaf7}}
\Delta \theta_i^{t+1}=-(\frac{1}{\alpha} \nabla_{\theta_i} F_i(\theta_i^{t+1})+h_i^t))=h_i^{t+1}-h_i^t
\end{equation}
Combine Equation \ref{lammaf7} and \ref{lammaf1}, the global parameter in the $t+1$ round is represented as
\begin{equation}{\label{lammaf8}}
\begin{split}
\Theta^{t+1}-\Theta^t&=\mathbb{E}(\theta_i^{t+1}+h_i^{t+1})-\Theta^t\\
&=\mathbb{E}(\Theta^t+\Delta \theta_i^{t+1}+ h_i^t+\Delta \theta_i^{t+1}-\Theta^t)\\
&=\mathbb{E}(2h_i^{t+1}-h_i^t)\\
&=-\frac{1}{\alpha} \mathbb{E}(2\nabla_{\theta_i} F_i(\theta_i^{t+1})-\nabla_{\theta_i} F_i(\theta_i^{t}))
\end{split}
\end{equation}
Besides, we also get
\begin{equation}{\label{lammaf9}}
\mathbb{E}(\theta_i^{t+1}-\theta_i^{t})
=\mathbb{E}(\Theta^{t+1}-\mathbb{E} h_i^{t+1})-\mathbb{E}(\Theta^{t}-\mathbb{E} h_i^{t})=\mathbb{E} h_i^{t+1}
\end{equation}

\textbf{Proof Convergence of FLN}
L-smooth
\begin{equation}{\label{lammaf10}}
f(y)\leq f(x)+<\nabla f(x),,y-x> +\frac{L}{2}||y-x||^2
\end{equation}
$\mu$ convex 
\begin{equation}{\label{lammaf10}}
f(y)\geq f(x)+<\nabla f(x),,y-x> +\frac{\mu}{2}||y-x||^2
\end{equation}

we get 
\begin{equation}{\label{lammaf10}}
\begin{split}
&\mathbb{E}F_i(\Theta^t)\leq \mathbb{E} F_i(\theta_i^t)+<\nabla F_i(\theta_i^t),\Theta^t-\theta_i^t>+\frac{L}{2}||\Theta_i^t-\theta_i^t||^2\\
&\mathbb{E}F_i(\Theta^t)\leq \mathbb{E} F_i(\theta_i^t)+<\nabla F_i(\theta_i^t),\Theta^t-\theta_i^t>+\frac{L}{2}||\Theta_i^t-\theta_i^t||^2\\
&\leq \mathbb{E} F_i(\theta_i^t)+(\frac{L}{2}-\alpha)||h_i^t||^2
\end{split}
\end{equation}
The clients using SGD in local training phase, we get $\mathbb{E}F_i(\theta_i^t)\leq \mathbb{E} F_i(\theta_i^{t,0})=\mathbb{E} F_i(\Theta^{t-1})$. So that 
\begin{equation}{\label{lammaf10}}
\begin{split}
&\mathbb{E}F_i(\Theta^t)- F_i(\Theta_i^{t-1})\leq \mathbb{E}(\frac{L}{2}-\alpha)||h_i^t||^2
\end{split}
\end{equation}

\textbf{Proof Convergence of FLN}

Suppose $L(\Theta)$ is a convex function, We choose the Regret statistic $R(T)$ to determine FLN's convergence, 
\begin{equation}{\label{lammaf10}}
R(T)=\sum_{t=1}^T L(\Theta^T)-\min_\Theta L(\Theta)
\end{equation}
When $T\rightarrow \infty$, if the average amortization value of $R(t)/T\rightarrow \infty$, the algorithm converged. At round $T$, the parameter of the global model minimize the objective function $\Theta^T\rightarrow \arg\min\sum_{t=1}^T L(\Theta^t)=^\triangleq \Theta^*$. Generally, the slower $R(T)$ increases with $T$, the faster the algorithm converges.

Because $\Theta^*=\arg\min_\Theta \sum_{t=1}^T L(\Theta)$, so
\begin{equation}{\label{lammaf11}}
R(T)=\sum_{t=1}^T L(\Theta^T)-\min_\Theta L(\Theta)=\sum_{t=1}^T [L(\Theta^T)-\min_\Theta L(\Theta)]
\end{equation}
$L$ is a convex function, we get 
\begin{equation}{\label{lammaf12}}
L(\Theta^*)\geq L(\Theta^t)+\langle \nabla L(\Theta^t),\Theta^*-\Theta^t\rangle \quad and \quad L(\Theta^t)-L(\Theta^*) \leq \langle \nabla L(\Theta^t),\Theta^*-\Theta^t \rangle
\end{equation}
%\begin{equation}{\label{lammaf12}}
%\nabla^{2} L(\Theta^t)>0 , \qquad \nabla L(\Theta^{t+1})= \nabla L(\Theta^t)+\nabla^{2} L(\Theta^t) (\Theta^{t+1}-\Theta^{t})
%\end{equation}

Take \ref{lammaf12} into $R(T)$, we get 
\begin{equation}{\label{lammaf13}}
R(T) \leq \sum_{t=1}^T \langle \nabla L(\Theta^t),\Theta^*-\Theta^t \rangle
\end{equation}

From the \ref{}, we get 
\begin{equation}{\label{lammaf13-1}}
\mathbb{E}\nabla F(\Theta^t)=\mathbb{E} \nabla F_i(\theta_i^t)
\end{equation}

We make a mathematical transformation of the iterative formula of $\Theta^t$ and suppose $g^{t}=((\nabla_{\theta_i} F_i(\theta_i^{t})+2\nabla_{\theta_i} F_i(\theta_i^{t+1})))$
\begin{equation}{\label{lammaf14}}
\begin{split}
&\Theta^{t+1}=\Theta^t-\frac{1}{\alpha} g^{t}\\
&\Rightarrow \Theta^{t+1}-\Theta^*=\Theta^t-\Theta^*-\frac{1}{\alpha} g^{t}\\
&\Rightarrow \Vert \Theta^{t+1}-\Theta^* \Vert_2^2=\Vert \Theta^{t}-\Theta^* \Vert_2^2-2\frac{1}{\alpha}\langle g^t, \Theta^t-\Theta^*\rangle +\frac{1}{\alpha^2}\Vert g^t \Vert_2^2\\
&\langle g^t, \Theta^t-\Theta^*\rangle = \frac{\alpha}{2} [ \Vert \Theta^{t}-\Theta^* \Vert_2^2- \Vert \Theta^{t+1}-\Theta^* \Vert_2^2 ] +\frac{1}{2\alpha}\Vert g^t \Vert_2^2
\end{split}
\end{equation}

$F$ is a $\mu$ convex function, so that 
\begin{equation}{\label{lammaf14-1}}
\begin{split}
&F(\Theta^*)\geq F(\Theta^t)+<\nabla F(\Theta^t),\Theta^*-\Theta^t>+\frac{\mu}{2}||\Theta^*-\Theta^t||^2\\
&F(\Theta^*)\geq F(\Theta^{t+1})+<\nabla F(\Theta^{t+1}),\Theta^*-\Theta^{t+1}>+\frac{\mu}{2}||\Theta^*-\Theta^{t+1}||^2\\
&\alpha<g,\Theta^t-\Theta^*>\\
&\geq 2F(\Theta^{t+1})-F(\Theta^t)-F(\Theta^*)+\mu||\Theta^*-\Theta^{t+1}||^2-\frac{\mu}{2}||\Theta^*-\Theta^{t}||^2-<\nabla F(\Theta^{t+1}),\Theta^{t+1}-\Theta^t>
\end{split}
\end{equation}

\begin{equation}{\label{lammaf14-2}}
\begin{split}
&||\Theta^*-\Theta^{t+1}||^2\leq \frac{1}{2}|\Theta^*-\Theta^{t}||^2+\\
&\frac{1}{\mu+1}
[\frac{(g^t)^2}{2}+(F(\Theta^t)-F(\Theta^*))-2(F(\Theta^{t+1})-F(\Theta^*))+<\Theta^{t+1},g^t>]
\end{split}
\end{equation}
where
\begin{equation}{\label{lammaf14-3}}
\begin{split}
&\frac{(g^t)^2}{2}+(F(\Theta^t)-F(\Theta^*))-2(F(\Theta^{t+1})-F(\Theta^*))+<\Theta^{t+1},g^t>\\
&=(F(\Theta^t)-F(\Theta^*))-2(F(\Theta^{t+1})-F(\Theta^*))+<\Theta^{t+1}+\frac{g^t}{2},g^t>\\
&\leq F( \Theta^t)+F(\Theta^*)-2F(\Theta^{t+1})+<\Theta^{t+1}+\frac{g^t}{2},g^t>\\
&\leq  F( \Theta^t)+F(\Theta^*)-2F( \Theta^t)-2\nabla F( \Theta^t)g^t+<\Theta^{t+1}+\frac{g^t}{2},g^t>\\
&\leq F(\Theta^*)-F( \Theta^t)-2\nabla F( \Theta^t)g^t+<\Theta^{t+1}+\frac{g^t}{2},g^t>\\
&\leq 0
\end{split}
\end{equation}

so that as $t\rightarrow \infty$, $\lim F(\Theta^t)-F(\Theta^*) =\frac{1}{2^T}(F(\Theta^0)-F(\Theta^*))\rightarrow 0$, the global model converges.

%%%%%%%%%%%%%%%%%%%%%%%%%%%%%%%%%%%%%%%%%%%%%%%%%%%%%%%
From \ref{lammaf14-1} and \ref{lammaf14}, we get 

So that 
\begin{equation}{\label{lammaf15}}
\begin{split}
R(T)&\leq \sum_{t=1}^T \{\frac{\alpha}{2} [ \Vert \Theta^{t}-\Theta^* \Vert_2^2- \Vert \Theta^{t+1}-\Theta^* \Vert_2^2 ] +\frac{1}{2\alpha}\Vert g^t \Vert_2^2\}\\
&=\sum_{t=1}^T \frac{\alpha}{2} [ \Vert \Theta^{t}-\Theta^* \Vert_2^2- \Vert \Theta^{t+1}-\Theta^* \Vert_2^2 ] +\sum_{t=1}^T \frac{1}{2\alpha}\Vert g^t \Vert_2^2\\
\end{split}
\end{equation}

\begin{equation}{\label{lammaf15}}
\begin{split}
2R(T+1)-R(T)&\leq \sum_{t+1}^T<g,\Theta^*>-\sum_{t+1}^T <\nabla L(\Theta^{t+1},\Theta^{t+1})>-2<\nabla L(\Theta^{T+1},\Theta^{T+1})>\\
&\sum_{t=1}^T \{\frac{\alpha}{2} [ \Vert \Theta^{t}-\Theta^* \Vert_2^2- \Vert \Theta^{t+1}-\Theta^* \Vert_2^2 ] +\frac{1}{2\alpha}\Vert g^t \Vert_2^2\}\\
&=\sum_{t=1}^T \frac{\alpha}{2} [ \Vert \Theta^{t}-\Theta^* \Vert_2^2- \Vert \Theta^{t+1}-\Theta^* \Vert_2^2 ] +\sum_{t=1}^T \frac{1}{2\alpha}\Vert g^t \Vert_2^2\\
\end{split}
\end{equation}

According to the gradient bound assumption, for the second part of \ref{lammaf15} we get 
\begin{equation}{\label{lammaf16}}
\sum_{t=1}^T \frac{1}{2\alpha}\Vert g^t \Vert_2^2 \leq \sum_{t=1}^T \frac{9}{2\alpha} G^2=\frac{9T}{2\alpha} G^2
\end{equation}
Performing the misalignment summation for the first part of \ref{lammaf15} we get 
\begin{equation}{\label{lammaf17}}
\begin{split}
&\sum_{t=1}^T \frac{\alpha}{2} [ \Vert \Theta^{t}-\Theta^* \Vert_2^2- \Vert \Theta^{t+1}-\Theta^* \Vert_2^2 ]\\
&=\frac{\alpha}{2} [ (\Vert \Theta^{1}-\Theta^* \Vert_2^2- \Vert \Theta^{2}-\Theta^* \Vert_2^2)+(\Vert \Theta^{2}-\Theta^* \Vert_2^2- \Vert \Theta^{3}-\Theta^* \Vert_2^2)\\
&+...+(\Vert \Theta^{T}-\Theta^* \Vert_2^2- \Vert \Theta^{T+1}-\Theta^* \Vert_2^2)]\\
&=\frac{\alpha}{2} [ \Vert \Theta^{1}-\Theta^* \Vert_2^2- \Vert \Theta^{T+1}-\Theta^* \Vert_2^2]\\
\end{split}
\end{equation}
According to the variable bounded assumption, we get
$\frac{\alpha}{2} [\Vert \Theta^{1}-\Theta^* \Vert_2^2] \leq \frac{\alpha}{2} D^2$ and $- \Vert \Theta^{T+1}-\Theta^* \Vert_2^2]\leq 0$. So that the upper bound of $R(T)$ is 
\begin{equation}\label{lammaf18}
R(T)\leq \frac{9T}{2\alpha} G^2+\frac{\alpha}{2} D^2
\end{equation}
The amortized value of $R(T)$ is $\frac{9}{2\alpha} G^2+\frac{\alpha D^2}{2T}$, the upper bound of $R(T)$ is $O(T)$, $R(T)/T$ converge to $\frac{9G^2}{2\alpha} $.

\section{Proof like FedDyn}

Define $C_t$ and
\begin{equation}\label{lammad18}
S^t=\mathbb{E}||\nabla F_i(\theta_i^t)-\nabla F_i(\Theta_*)||^2, \quad \varepsilon^t=\mathbb{E}||\theta_i^t-\Theta^{t-1}||^2=\mathbb{E}||h_i^t-h_i^{t-1}||^2=\mathbb{E}||\Delta \theta_i^t||^2
\qquad \varepsilon^t=\mathbb{E}||\theta_i^t-\bar\theta^{t-1}||^2
\end{equation}

Lemma 2
\begin{equation}\label{lammad18}
\mathbb{E} [\Theta^t-\Theta^{t-1}]=\mathbb{E}(2h_i^t-h_i^{t-1})=\frac{1}{\alpha}\mathbb{E}[-2\nabla F_i(\theta_i^t)+\nabla F_i(\theta_i^{t-1})]
\end{equation}

\begin{equation}\label{lammad18}
\mathbb{E} [\theta_i^{t+1}-\hat\theta_i^{t}]= \frac{1}{\alpha}[-\nabla L_i(\theta_i^{t+1})]
\end{equation}

\textcolor{red}{text}Lemma 3
\begin{equation}\label{lammad18}
\mathbb{E} ||\Theta^{t+1}-\Theta^{t}||^2\leq 4(h_i^{t+1})^2+(h_i^t)^2-4h_i^{t+1}h_i^t
\end{equation}
\begin{equation}\label{lammad18}
\mathbb{E} ||\theta_i^{t+1}-\hat\theta_i^{t}||^2\leq \varepsilon^{t+1}
\end{equation}

Lemma 5
\begin{equation}{\label{lammaf15}}
\begin{split}
\mathbb{E}||\Theta^{t+1}-\Theta^*||^2& = \mathbb{E}||\Theta^{t}-\Theta^*+\Theta^{t+1}-\Theta^{t}||^2\\
&=\mathbb{E}\mathbb{E}||\Theta^{t}-\Theta^*||^2+\mathbb{E}||\Theta^{t+1}-\Theta^t||^2+2\mathbb{E}<\Theta^t-\Theta^*,\Theta^{t+1}-\Theta^t>\\
&=-2\frac{1}{\alpha} \mathbb{E}<\Theta^t-\Theta^*,(2\nabla_{\theta_i} F_i(\theta_i^{t+1})-\nabla_{\theta_i} F_i(\theta_i^{t}))>+\mathbb{E}||\Theta^{t}-\Theta^*||^2+\mathbb{E}||\Theta^{t+1}-\Theta^t||^2\\
&=\frac{2}{\alpha} \mathbb{E}[F_i(\Theta^*)-F_i(\Theta^{t})+L||\theta_i^{t+1}-\Theta^t||^2-\frac{L}{2}||\theta_i^{t}-\Theta^t||^2]+\mathbb{E}||\Theta^{t}-\Theta^*||^2+\mathbb{E}||\Theta^{t+1}-\Theta^t||^2\\
&=\mathbb{E}||\Theta^{t}-\Theta^*||^2+\mathbb{E}||\Theta^{t+1}-\Theta^t||^2+\frac{2}{\alpha}\mathbb{E} [F(\Theta^t)-F(\Theta^*)]+\frac{L}{\alpha}(2\varepsilon^{t+1})-\mathbb{E}\frac{L}{\alpha}||\theta_i^{t}-\Theta^t||^2\\
&=\mathbb{E}||\Theta^{t}-\Theta^*||^2+\mathbb{E}||\Theta^{t+1}-\Theta^t||^2+\frac{2}{\alpha}\mathbb{E} [F(\Theta^t)-F(\Theta^*)]+\frac{L}{\alpha}[2(h_i^{t+1})^2+(h_i^t)^2-4h_i^{t+1}h_i^t]\\
&=\mathbb{E}||\Theta^{t}-\Theta^*||^2+\frac{2}{\alpha}\mathbb{E} [F(\Theta^t)-F(\Theta^*)]\\
&+[(\frac{2L}{\alpha}+4)(h_i^{t+1})^2+(\frac{L}{\alpha}+1)(h_i^t)^2-(\frac{4L}{\alpha}+4)h_i^{t+1}h_i^t]
\end{split}
\end{equation}

Lemma 6

Lemma 7

Proof of Lemma 4
\begin{equation}{\label{lammaf15}}
\varepsilon^t=\mathbb{E}||\theta_i^t-\Theta^{t-1}||^2=\mathbb{E}||h_i^t-h_i^{t-1}||^2=\mathbb{E}[(h_i^t)^2-2h_i^th_i^{t-1}+(h_i^{t-1})^2]
\end{equation}

Proof of Lemma 5
\begin{equation}{\label{lammaf15}}
S^t=\mathbb{E}||\nabla F_i(\theta_i^t)-\nabla F_i(\Theta_*)||^2
\leq (1-\frac{P}{m})S_{t-1}+\frac{2L^2P}{m}\varepsilon^t+\frac{4LP}{m}\mathbb{E} [F(\Theta^{t-1})-F(\Theta^*)]
\end{equation}
